# Supplementary material for: Surface hopping methodology in laser-driven molecular dynamics
Source: arXiv:1608.08768 ancillary file (2016-09-01)
Supplement: Supplementary file 1 [file supplement.pdf]

# Supplemental material to "Surface hopping methodology in laser-driven molecular dynamics"

T. Fiedlschuster,[1,2] J. Handt,[1] E.K.U. Gross,[2] and R. Schmidt[1]

[1]*Institut für Theoretische Physik, Technische Universität Dresden, D-01062 Dresden, Germany*
[2]*Max-Planck-Institut für Mikrostrukturphysik, Weinberg 2, D-06120 Halle, Germany*

(Dated: August 23, 2016)

In this supplemental material, we give some general information about the investigated scenarios (Sec. I), numerical details concerning the solution of the time-dependent Schrödinger equation (TDSE, Sec. II), details of the calculation of the exact potential energy surface (EPES) from the full electron-nuclear wave function (Sec. III), as well as details regarding the quantum-classical methods (Sec. IV), in particular the surface hopping methods (Sec. IV A) and the exact surface dynamics (ESD) (Sec. IV B). Furthermore, to visualize the time-dependence of the different potential energy surfaces, we provide and discuss several movies (Sec. V).

## I. DETAILS FOR SCENARIO 1 AND 2

To validate surface hopping for laser-driven molecular dynamics and to unambiguously demonstrate the differences between surface hopping using Born-Oppenheimer surfaces (BOSs), instantaneous BOSs (IBOSs), and Floquet surfaces (FSs), we performed exemplary calculations and compared the resulting nuclear probability density distributions (NPDDs). The chosen scenarios are hand-picked to support our statements while being clear, vivid, and not too specific, i.e., they represent generic scenarios of molecular dissociation.

*Scenario 1 (photon absorption)* The first scenario is designed to steer the molecule into the bond softening dissociation channel. The molecule initially is in the electronic ground state. The nuclei are in an excited state constructed by providing an additional momentum of $-2.5$ a.u. to the vibrational ground state $\nu = 0$. Due to this initial nuclear excitation, the dissociating part of the NPDD forms a peak (see Fig. 2 in the article), which makes the example generally more significant. Pronounced bond softening dissociation also could be reached by starting with certain excited vibrational states, which, unfortunately, is problematic in our quantum-classical calculations (see Sec. IV C).

*Scenario 2 (photon emission)* The second scenario is designed to make hops in F-SH *inevitable* for an agreement to the TDSE dynamics. The molecule starts in an electronic excited state (first excited BO state), the initial state of the nuclei is the Franck-Condon projection of the vibrational ground state $\nu = 0$ onto the eigenstates of the nuclei in the potential energy surface of the excited electronic state. The laser envelope is tuned such that the wave packet passes the one-photon resonance when the maximal intensity is reached, which itself is chosen such that the wave packet splits into two nearly equal parts during the dynamics. For the Floquet picture to approximately apply, the pulse envelope must not change too drastically during one optical cycle of the laser. For the $H_2^+$-like model, where the one-photon resonance is reached very quickly, the approximate validity of the Floquet picture is questionable. To counter this, we use a $Na_2^+$-like model with larger nuclear mass in scenario 2. The slower nuclear dynamics allows us to stretch the pulse envelope, fitting much more optical cycles into it.

## II. NUMERICAL SOLUTION OF THE TDSE

We solve the TDSE

$$i\partial_t \psi(R, r, t) = H(R, r, t)\psi(R, r, t) \tag{1}$$

for the model system defined by the Hamiltonian

$$\begin{aligned} H = &- \frac{\Delta_R}{2M} - \frac{\Delta_r}{2} + \frac{1}{R + 0.03} - \mu F(t) cos(\omega t) \\ &- \frac{1}{\sqrt{(r - R/2)^2 + 1}} - \frac{1}{\sqrt{(r + R/2)^2 + 1}} \end{aligned} \tag{2}$$

(see Eq. (1) in our article) using the second order split-operator method on a grid. The grid spans from $R = 0$ a.u. to $R = 20$ a.u. for the nuclear bond length and from $r = -20$ a.u. to $r = 20$ a.u. for the electron. This small grid is sufficient for the investigated examples. To prevent unphysical reflections, the values of the wave function near the grid boundaries are damped by an absorber function. For the $H_2^+$-like model ($M = 918$ a.u.), we use 512 grid points for the electron as well as the nuclei. For the $Na_2^+$-like model ($M = 23 \times 918$ a.u.), we use 512 grid points for the electron and 16.384 grid points for the nuclei. The relatively large number of nuclear grid points is due to the larger nuclear momenta and necessary for convergence of the EPES calculation (see Sec. III). We use a time step of $\Delta t = 0.1$ a.u. in all cases.

## III. CALCULATION OF THE EPES

The EPES is calculated by factorizing the full electron-nuclear wave function (see [1, 2])

$$\psi(R, r, t) = \chi(R, t)\phi_R(r, t), \tag{3}$$

with

$$\chi(R,t) = e^{\mathrm{i}S(R,t)}\sqrt{\int dr\ |\psi(R,r,t)|^2}, \tag{4}$$

and

$$\phi_R(r,t) = \frac{\psi(R,r,t)}{\chi(R,t)}. \tag{5}$$

The phase $S(R,t)$ is determined in a gauge with vanishing vector potential

$$A(R,t) = -\mathrm{i}\int dr\ \phi_R^*(r,t)\partial_R\phi_R(r,t) = 0, \tag{6}$$

and reads

$$S(R,t) = \int_{R_0}^{R} dR' \frac{Im\left\{\int dr\ \psi(R',r,t)\partial_{R'}\psi(R',r,t)\right\}}{|\chi(R',t)|^2}. \tag{7}$$

In the same gauge, the EPES is calculated as

$$\epsilon(R,t) = \mathrm{i}\frac{\partial_t\chi(R,t)}{\chi(R,t)} + \frac{\Delta_R\chi(R,t)}{2M\chi(R,t)}. \tag{8}$$

Since $A = 0$, the exact force is given by the gradient of the EPES alone. With $A = 0$, the EPES may still be shifted (globally) by a constant to fix the gauge entirely. In Figs. 2 and 4 of our article, we use this to shift the EPES to the Floquet surfaces. For the comparison of Floquet surfaces and EPES, the latter is averaged over one optical cycle of the laser $T = 2\pi/\omega \approx 0.8$ fs. The averaged EPES reads

$$\tilde{\epsilon}(R,t) = \frac{1}{T}\int_{-T/2}^{T/2} dt'\ \epsilon(R,t). \tag{9}$$

The difference between $\epsilon$ and $\tilde{\epsilon}$ mainly consists in an oscillation of $\epsilon$ around $\tilde{\epsilon}$ with twice of the laser frequency and a $R$-dependent amplitude (see Sec. V).

## IV. MIXED QUANTUM-CLASSICAL METHODS

### A. Details for the surface hopping schemes

In our article, we compare three different hopping methods, namely

- BO-SH: hopping between BOSs (obtained by diagonalizing the field-free electronic Hamiltonian)
- IBO-SH: hopping between IBOSs (obtained by diagonalizing the BO Hamiltonian including the interaction with the classical laser field)
- F-SH: hopping between FSs (obtained by diagonalizing the BO Hamiltonian including the quantized, photon-resolved laser-molecule interaction [3, 4])

In all cases, an ensemble of $N = 100.000$ independent classical trajectories $R(t)$ is propagated on potential energy surfaces (PES) to mimic the quantum-mechanical wave packet dynamics. The large number of trajectories is not necessary for convergence, but favorable for binning and displaying the resulting nuclear probability densities. For the classical initial conditions see Sec. IV C. The trajectories are propagated using the leap-frog algorithm with a time step $\Delta t = 0.01$ a.u. Simultaneously, for each trajectory, a TDSE for the electron is solved in basis expansion to determine the hopping probability. The electronic wave function is expanded into the two lowest BO states (BO-SH and IBO-SH) or into dressed BO states (F-SH, see [5]). This wave function is then transformed into the basis of IBO states for IBO-SH, and into Floquet states for F-SH. Following Tully's fewest switching algorithm [6], the time-evolution of the electronic wave function determines the hopping probability between different PES. We do not repeat the explicit calculation of the hopping probabilities here, the interested reader may have a look at [7] for BO-SH, [8, 9] for IBO-SH, and [5] for F-SH. In addition to the differences of the applied PES, the hopping methods differ considerably in the way how hops are performed.

- If a hop occurs in BO-SH, the trajectory is set onto the new BO surface. The momentum of the trajectory is strictly conserved, assuming that the energy difference before and after the hop is provided by the laser field.
- If a hop occurs in F-SH, the trajectory is set onto the new Floquet surface. The laser-molecule interaction is incorporated into the Floquet surfaces, thus the energy is strictly conserved. The momentum after the hop is adjusted to match the new kinetic energy. If a hop would result in negative kinetic energy, it is considered "classically forbidden" and rejected.
- If a hop occurs in IBO-SH, the trajectory is set onto the new IBO surface. The use of IBO-SH comes with some peculiarities concerning energy and momentum conservation. We apply the "ratio method," developed in [9]. This method proposes a "weighted conservation" of energy and momentum, based on the ratio of different contributions to the hopping probability (see Sec. 3 in [9]). The ratio method manages to connect special cases of strict momentum and strict energy conservation, resulting, however, in neither strict momentum nor strict energy conservation for most cases. Hops which result in negative kinetic energy are rejected.

### B. Details for the exact surface dynamics (ESD)

For the propagation of classical trajectories on the EPES (see Sec. III) the same initial conditions and numerical parameters as for the surface hopping methods

are used (see Sec. IV A). We note that, for the chosen laser parameters and nuclear masses, the nuclear probability densities obtained with classical trajectories propagated on the EPES $\epsilon$ and the time-averaged EPES $\tilde{\epsilon}$ (see (8) resp. (9)) are practically identical.

### C. Classical initial conditions

In our article, we compare the quantum-classical nuclear probability densities (NPDDs) with the exact quantum-mechanical NPDD (obtained by solving the TDSE), which comes with some constraints in the initial conditions. The appropriate choice of initial conditions for an ensemble of classical nuclear trajectories in a quantum-classical calculation is a fundamental question of general interest, which we do not want to address here. Focusing on the NPDD as observable, however, the initial conditions must lead to a quantum-classical NPDD identical to the NPDD of the corresponding quantum state, at $t = 0$. A way to satisfy this is to sample the classical initial conditions (in phase space $\{R,\ P\}$) from the Wigner distribution of the initial nuclear quantum state $\varphi(R, t_0)$,

$$W_{\varphi(t_0)}(R,P) = 2\pi \int dQ\, e^{-\mathrm{i}PQ} \varphi(R+\frac{Q}{2}, t_0)\varphi^*(R-\frac{Q}{2}, t_0). \quad (10)$$

The reader not familiar with the Wigner distribution is encouraged to have a look at [10]. $W(R,P)$ fulfills

$$\int dP\ W_{\varphi(t)}(R,P) = |\varphi(R,t)|^2 \quad (11)$$

and

$$\int dR\ W_{\varphi(t)}(R,P) = |\varphi(P,t)|^2, \quad (12)$$

such that the resulting NPDDs, in position space as well as in momentum space, are identical. The time-dependent Wigner distribution can be obtained by solving the TDSE for the corresponding state $|\varphi(t)\rangle$, or by solving the Wigner-Liouville equation for $W_{\varphi(t=0)}(R,P)$.

In Fig. 1, the Wigner distributions of the first four vibrational states for our $H_2^+$-like model are shown. It becomes apparent that the phase space distribution $W(R,P)$ is remarkably different compared to the phase space accessible by a classical trajectory, propagated in the ground state BOS with the corresponding vibrational energy $E_\nu$. Fig. 1 furthermore reveals that the Wigner distribution is negative in wide phase space regions for $\nu = 1, 2, 3$. These large regions of negative values are well understandable, since the Wigner distributions of orthogonal quantum states are orthogonal,

$$\langle\varphi_1|\varphi_2\rangle = 0 \Leftrightarrow \int dR\ dP\ W_{\varphi_1} W_{\varphi_2} = 0. \quad (13)$$

Thus, with the positive Wigner distribution of the vibrational ground state $\nu = 0$, the Wigner distributions of all excited vibrational states will take negative values in considerable phase space volumes to satisfy (13). The role of positive and negative values in $W(R,P)$ is crucial when calculating observables, e.g., (11) and (12). Even in cases where the full Wigner-Liouville dynamics only marginally deviates from purely classical dynamics, the balance of "positive" and "negative" trajectories is disturbed. The predictions for observables, calculated by an ensemble of classical trajectories, become physically meaningless. This restricts us to initial quantum states with positive Wigner distributions, e.g., the vibrational ground state $\nu = 0$.

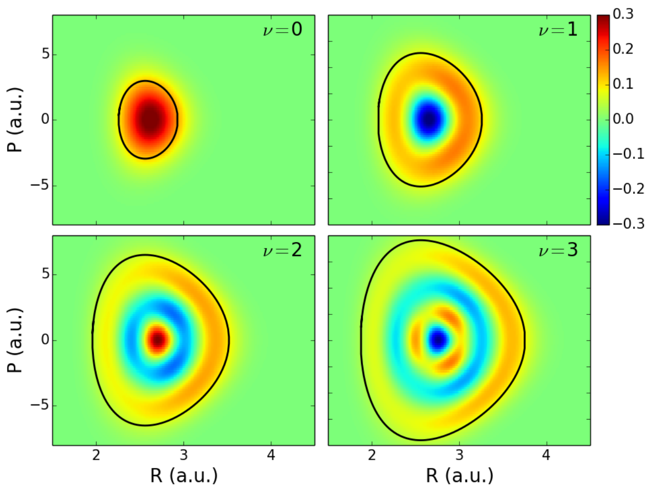


FIG. 1. The Wigner distribution for the vibrational states $\nu = 0, 1, 2, 3$ for the $H_2^+$-like model. The black line shows the accessible phase space for a classical trajectory with the corresponding vibrational energy $E_\nu$.

## V. VISUALIZATION OF PES AND NPPDs (MOVIES)

In this section, we discuss the movies provided with this supplemental material.

*1.* The movie "figure1.mov" is a time-dependent version of Fig. 1 of our article. It shows BO, IBO, and Floquet surfaces for the $H_2^+$-like model system for the first 10 fs of the laser used in scenario 1. The differences between the surfaces (time-independent BO surfaces, slowly time-dependent Floquet surfaces, and rapidly oscillating IBO surfaces) are apparent.

*2.* The movie "scenario1.mov" is a time-dependent version of Fig. 2 of our article. It shows the time-dependent NPDD, obtained by solving the TDSE, alongside with the ground state BO surface and the Floquet

surface relevant for one-photon dissociation. The EPES as well as the EPES averaged over one optical cycle of the laser are shown in regions of non-vanishing NPDD. While the oscillation of the EPES is similar to that of the IBO surfaces, the shape of the EPES is already clearly comparable to the Floquet surface. Averaging the EPES over one optical cycle yields a surface remarkably close to the Floquet surface, in shape and time dependence. For the chosen nuclear mass and laser parameters, the oscillation of the EPES has practically no impact on the classical nuclear dynamics.

*3.* The movie "scenario2.mov" is a time-dependent version of Fig. 4 of our article. Also this movie shows the time-dependent NPDD, obtained by solving the TDSE, alongside with the ground state BO surface and the two relevant Floquet surfaces. The EPES in regions of non-vanishing NPDD is shown twice, clamped at the different Floquet surfaces. After the NPDD passed the region of resonant one-photon emission, the EPES forms a cone, actively splitting the classical NPDD propagated on it (not shown) into the two peaks also observed in the exact TDSE dynamics. The gradient of the EPES left/right of the cone is practically identical to the gradient of the upper/lower Floquet surface. As shown in our article, F-SH also yields the correct splitting, due to the hopping during the laser pulse.


[1] A. Abedi, N. T. Maitra, and E. K. U. Gross, Phys. Rev. Lett. **105**, 123002 (2010).
[2] A. Abedi, N. T. Maitra, and E. K. U. Gross, The Journal of Chemical Physics **137**, 22A530 (2012).
[3] H. Sambe, Phys. Rev. A **7**, 2203 (1973).
[4] S. Guerin, F. Monti, J.-M. Dupont, and H. R. Jauslin, J. Phys. A: Math. Gen. **30**, 7193 (1997).
[5] T. Fiedlschuster, J. Handt, and R. Schmidt, Phys. Rev. A **93**, 053409 (2016).
[6] J. C. Tully, J. Chem. Phys. **93**, 1061 (1990).
[7] M. Fischer, J. Handt, and R. Schmidt, Phys. Rev. A **90**, 012525 (2014).
M. Fischer, J. Handt, and R. Schmidt, Phys. Rev. A **90**, 012526 (2014).
M. Fischer, J. Handt, and R. Schmidt, Phys. Rev. A **90**, 012527 (2014).
[8] M. Thachuk, M. Y. Ivanov, and D. M. Wardlaw, J. Chem. Phys. **105**, 4094 (1996).
[9] M. Thachuk, M. Y. Ivanov, and D. M. Wardlaw, J. Chem. Phys. **109**, 5747 (1998).
[10] W. B. Case, American Journal of Physics **76**, 937 (2008).
